# Supplementary material for: An elementary introduction to information geometry
Source: arXiv:1808.08271 source file (2020-09-06)
Supplement: Supplementary file 1 [file Appendix-GaussianFamily.tex]

%%%%
\section{Expected $\alpha$-geometry of the Gaussian family}
%%%%

Consider the family of univariate Gaussian distributions: 
\begin{equation}
\calN \eqdef \{ p_\lambda(x,\lambda) \st \lambda\in\bbR\times \bbR^+ \},
\end{equation}
with
\begin{equation}
p_\lambda(x,\lambda=(\lambda_1=\mu,\lambda_2=\sigma^2)) =  \frac{1}{\sqrt{2\pi\lambda_2}} \exp(-\frac{(x-\lambda_1)^2)}{2\lambda_2}).
\end{equation}
We can rewrite the normal density into the canonical representation of an exponential family:
\begin{equation}
\log p_\theta(x, \theta) =  \theta_1 x+\theta_2 x^2 - F_\calN(\theta),
\end{equation}
with
\begin{eqnarray}
\theta_1 &=& \frac{\mu}{\sigma^2}=\frac{\lambda_1}{\lambda_2},\\
\theta_2 &=& -\frac{1}{2\sigma^2}=-\frac{1}{2\lambda_2},\\
F_\calN(\theta) &=& -\frac{\theta_1^2}{4\theta_2}+ \frac{1}{2}\log(-\frac{\pi}{\theta_2}).
\end{eqnarray}
The exponential family of univariate Gaussian distributions is: 
\begin{equation}
\calN = \{ p_\theta(x,\theta) \st \theta\in\bbR\times \bbR^- \},
\end{equation}
and  we have $p_\lambda(x,\lambda)=p_\theta(x,\theta(\lambda))$ and $p_\theta(x,\theta)=p_\lambda(x,\lambda(\theta))$, with the
following invertible conversion functions:
\begin{eqnarray}
\theta(\lambda) &=& \left(\frac{\lambda_1}{\lambda_2},-\frac{1}{2\lambda_2}\right),\\
\lambda(\theta) &=& \left(-\frac{\theta_1}{2\theta_2}, -\frac{1}{2\theta_2} \right).
\end{eqnarray}

The Fisher information matrix (FIM) $\leftsub{\calN}I^\theta$ with respect to the natural parameters $\theta$ is given by the hessian of the potential function $F_\calN(\theta)$:
\begin{equation}
\leftsub{\calN}I_{ij}^\theta(\theta)  = \partial_i\partial_j F_\calN(\theta).
\end{equation}
Calculations yield:
\begin{equation}
\leftsub{\calN}I_{ij}^\theta(\theta)  =   \mattwotwo{-\frac{1}{2\theta_2}}{\frac{\theta_1}{2\theta_2^2}}{\frac{\theta_1}{2\theta_2^2}}{\frac{\theta_2-\theta_1^2}{2\theta_2^3}}.
\end{equation}
We can express this FIM using the $\lambda$ parameters as:
\begin{equation}
\leftsub{\calN}I_{ij}^\theta(\lambda(\theta))  =   \mattwotwo{\sigma^2}{2\mu\sigma^2}{2\mu\sigma^2}{2\sigma^2(2\mu^2+\sigma^2)}.
\end{equation}
We can also calculate the FIM with respect to the $\lambda$ parameters:
\begin{equation}
\leftsub{\calN}I_{ij}^\lambda(\lambda)  = \mattwotwo{\frac{1}{\sigma^2}}{0}{0}{\frac{1}{2\sigma^2}}.
\end{equation}
We check that the FIM is covariant by reparameterization:
\begin{equation}
\leftsub{\calN}I^\lambda(\lambda)  = J^{\theta\lambda}^\top \leftsub{\calN}I^\theta(\theta(\lambda)) J^{\theta\lambda},
\end{equation}
where $J$ is the Jacobian matrix of first derivatives: 
\begin{equation}
J^{\theta\lambda}_{ij}=\frac{\partial \theta_i}{\partial\lambda_j}.
\end{equation}

The dual Legendre potential function is
\begin{equation}
F^*(\eta)=-\frac{1}{2}\log (n_1^2-\eta_2),
\end{equation}
with $\eta=\nabla F(\theta)=(-\frac{\theta_1}{2\theta_2}, -\frac{1}{2\theta_2}+\frac{\theta_1^2}{4\theta_2^2})$.

The entropy, cross-entropy and Kullback-Leibler divergence between two Gaussian distributions is:
\begin{eqnarray}
h(p_\theta(x;\theta)) &=&,\\
h^\cross(p_\theta(x;\theta_1):p_\theta(x;\theta_2)) &=&,\\
\KL(p_\theta(x;\theta_1):p_\theta(x;\theta_2)) &=& .
\end{eqnarray}

We can use the mixed coordinates $(\theta_1,\eta_2)$ and $(\eta_1,\theta_2)$ to get a diagonal representation of the FIM that corresponds to orthogonal foliations.
...

\begin{eqnarray}
p_{m_1}(x;(\eta_1,\theta_2)) &=&,\\
p_{m_2}(x;(\eta_1,\theta_2)) &=&\sqrt{-\frac{\theta_2}{\pi}}\exp((x-\eta_1)^2\theta_2).\\
\end{eqnarray}

The expected $\alpha$-connections are given by
\begin{eqnarray}\label{eq:}
\Gamma_{11,1} &=& \\
\Gamma_{11,2} &=& \frac{1-\alpha}{\sigma^3} \\
\Gamma_{12,1} &=& -\frac{1+\alpha}{\sigma^3} \\
\Gamma_{11,2} &=& \\
\Gamma_{21,1} &=& \\
\Gamma_{21,2} &=&   \\
\Gamma_{22,1} &=&   \\
\Gamma_{21,2} &=& -\frac{2+4\alpha}{\sigma^3} \\
\end{eqnarray}

The $\alpha$-curvature tensor is given by
\begin{eqnarray}
R_{1212}^\alpha=\frac{1-\alpha^2}{\sigma^4},\quad R_{ijkl}^\alpha=0 (i,j,k,l)\not =(1,2,1,2).
\end{eqnarray}

The $\alpha$-Gaussian curvature is:
\begin{eqnarray}
K^\alpha = \frac{\alpha^2-1}{2}
\end{eqnarray}

Notice that all the above computations can be carried out using a computer algebra system like Maxima\footnote{\url{http://maxima.sourceforge.net/}}.
